# Supplementary material for: Direct and converse flexoelectricity in two-dimensional materials
Source: arXiv:2010.08470 ancillary file (2021-10-15)
Supplement: Supplementary file 1 [file supp.pdf]

# Supplemental Material for "Direct and converse flexoelectricity in two-dimensional materials"

Matteo Springolo, Miquel Royo and Massimiliano Stengel

October 4, 2021

## Contents

**1 Introduction** **2**

**2 Strain field near a curved surface** **2**
2.1 Nanotube geometry . . . . . . . . . . . . . . . . . . . . . . . . . . . . . 2
2.2 Flexural phonons . . . . . . . . . . . . . . . . . . . . . . . . . . . . . . 3

**3 Microscopic response in curvilinear coordinates** **4**

**4 Clamped-ion and lattice-mediated coefficients** **6**
4.1 Bulk flexoelectric tensor in 3D . . . . . . . . . . . . . . . . . . . . . . 6
4.2 Gradient contribution . . . . . . . . . . . . . . . . . . . . . . . . . . . 7
4.3 Uniform strain contribution . . . . . . . . . . . . . . . . . . . . . . . . 8
4.4 Total open-circuit voltage response . . . . . . . . . . . . . . . . . . . . 9
4.5 The longitudinal case . . . . . . . . . . . . . . . . . . . . . . . . . . . 11

**5 Computational parameters** **12**
5.1 Primitive-cell linear-response calculations . . . . . . . . . . . . . . . . 12
5.2 Direct nanotube calculations . . . . . . . . . . . . . . . . . . . . . . . 12

**6 Supplemental results** **14**
6.1 Analysis of the clamped-ion contribution . . . . . . . . . . . . . . . . . 14
6.2 Analysis of the lattice-mediated contribution . . . . . . . . . . . . . . 14
6.3 Generalized-gradient approximation . . . . . . . . . . . . . . . . . . . 16
6.4 Comparison to the literature . . . . . . . . . . . . . . . . . . . . . . . 16

**7 An illustrative toy model: Xe monolayer** **17**

**8 Coupling between out-of-plane electric fields and flexural phonons** **21**
8.1 Macroscopic electric fields in 2D . . . . . . . . . . . . . . . . . . . . . 21
8.2 Flexovoltage . . . . . . . . . . . . . . . . . . . . . . . . . . . . . . . . 22
8.3 Converse flexoelectric effect in 2D . . . . . . . . . . . . . . . . . . . . 22
8.4 Continuum modeling of PFM experiments . . . . . . . . . . . . . . . . 23

# 1 Introduction

Here we shall provide additional details in support of the results of the main text. In Sec.2 we explicitly derive the strain field acting on a bent layer, either in a nanotube geometry or in the case of a flexural phonon. In Sec. 3 spell out the derivation of the "local piezoelectricity" (U), "local flexoelectricity" (G) and "metric" (M) contributions to the flexovoltage, Eq. (3–8). In Sec. 4 we demonstrate the decomposition into clamped-ion (CI) and lattice-mediated (LM) effects of Eq. (9–11); we also derive the (vanishing) longitudinal coefficient via a closely related formula, which we use as a numerical consistency check. In Sec. 5 we describe the computational parameters and approximations that we used in the calculations. In Sec. 6 we provide additional results and data in support of our conclusions: (i) we decompose the CI values of Table I into the individual contributions described in the text; (ii) we analyze the LM contribution to the response in physically intuitive terms; (iii) we present a "toy model" consisting of a hexagonal monolayer of Xe atoms, which reduces to an analytically solvable system of noninteracting spheres in the limit of a large lattice parameter. Finally, in Sec. 8 we establish the formal relation between the 2D flexoelectric coefficient as defined in the main text and the coupling between flexural distortions of the flat layer and inhomogeneous out-of-plane electric fields. We also present a numerical validation of the converse flexoelectric effect by using BN as a testcase, and we discuss the practical application of our results to the interpretation of typical piezo-force microscopy (PFM) experiments.

# 2 Strain field near a curved surface

## 2.1 Nanotube geometry

We shall consider the mechanical deformation illustrated in Fig. 1, which corresponds to folding a flat monolayer into a cylindrical nanotube geometry. This transformation of the crystal is conveniently described by a mapping between a curvilinear and Cartesian frame of the type

$$x = (\xi_3 + R)\sin\left(\frac{\xi_1}{R}\right), \tag{1a}$$

$$z = (\xi_3 + R)\cos\left(\frac{\xi_1}{R}\right) - R, \tag{1b}$$

where $\xi_3$ spans the radial direction, while $\xi_1$ runs over the tangential direction. In the limit of large $R$, in a neighborhood of the origin we have immediately

$$x \simeq \xi_1 + \frac{\xi_1\xi_3}{R}, \tag{2a}$$

$$z \simeq \xi_3 - \frac{\xi_1^2}{2R}, \tag{2b}$$

corresponding to a macroscopic transverse strain gradient that is proportional to $1/R$.

For a more rigorous derivation, one can define the deformation gradient as

$$h_{\alpha\beta} = \frac{\partial r_\alpha}{\partial \xi_\beta}, \qquad \mathbf{h} = \begin{vmatrix} \frac{\xi_3+R}{R}\cos\left(\frac{\xi_1}{R}\right) & \sin\left(\frac{\xi_1}{R}\right) \\ -\frac{\xi_3+R}{R}\sin\left(\frac{\xi_1}{R}\right) & \cos\left(\frac{\xi_1}{R}\right) \end{vmatrix} \tag{3}$$

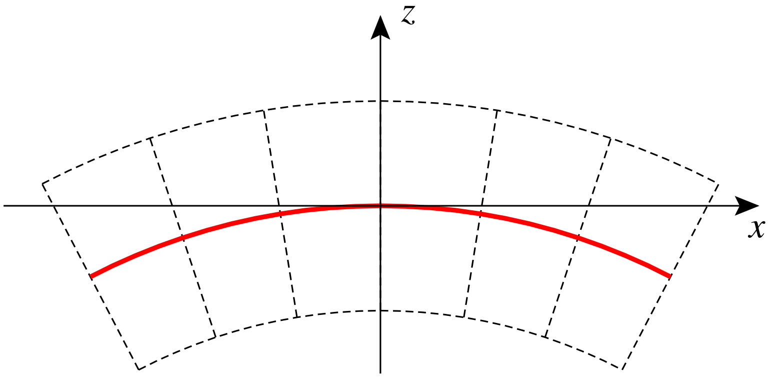


Figure 1: Illustration of the macroscopic deformation field in a vicinity of a bent layer; the two-dimensional crystal is indicated by a thicker red curve.

The metric tensor of the deformation is then defined by

$$\mathbf{g} = \mathbf{h}^{\mathrm{T}}\mathbf{h}, \qquad \mathbf{g} = \begin{vmatrix} \frac{(\xi_3+R)^2}{R^2} & 0 \\ 0 & 1 \end{vmatrix}. \tag{4}$$

The Lagrange strain tensor is defined in terms of the metric tensor as

$$\boldsymbol{\varepsilon} = \frac{1}{2}(\mathbf{g}-\mathbf{I}), \qquad \boldsymbol{\varepsilon} \simeq \frac{1}{R}\begin{vmatrix} \xi_3 & 0 \\ 0 & 0 \end{vmatrix}, \tag{5}$$

where in the second equality we have assumed that $\xi_3/R$ is a small number, consistent with the large-$R$ limit that is implicit in our theory. We obtain a linear variation of $\varepsilon_{xx}$ along the out-of-plane coordinate, thus proving our point. Similar conclusions were reached in Ref. [1].

## 2.2 Flexural phonons

Consider a long-wavelength phonon traveling in-plane at some wavevector $\mathbf{q}$ in a 2D crystal. In the linear regime, the corresponding atomic displacement pattern can be written as a cell-periodic part times a phase,

$$u^l_{\kappa\beta} = u^{\mathbf{q}}_{\kappa\beta} e^{i\mathbf{q}\cdot\mathbf{R}_{l\kappa}}, \tag{6}$$

where $\mathbf{R}_{l\kappa}$ is the position of the atom $l\kappa$ at rest. Flexural phonons are defined by their small-momentum behavior, which tends to a rigid translation of the crystal along the out-of-plane direction, $z$,

$$u^{\mathbf{q}}_{\kappa\beta} = U\left(\delta_{\beta z} + iq_\gamma \Gamma^\kappa_{\beta z\gamma} - q_\gamma q_\sigma N^\kappa_{\beta z,\gamma\sigma} + \cdots\right). \tag{7}$$

Higher-order terms correspond to the atomic distortions produced by a uniform strain $\varepsilon_{z\gamma}$ and a (type-I) strain gradient $\eta_{z,\gamma\sigma}$, respectively [2].

For a free-standing layer, the "uniform strain" response is determined by rotational invariance, [3, 4]

$$\Gamma^\kappa_{\beta z\gamma} = -\delta_{\beta\gamma}\tau_{\kappa z}, \tag{8}$$

where $\boldsymbol{\tau}_\kappa$ is the unperturbed location of atom $\kappa$. Equivalently, we can write the macroscopic displacement field in a vicinity of the layer plane as

$$u_\beta(\mathbf{r}) = U\left(\delta_{\beta z} - iq_\gamma \delta_{\beta\gamma} z\right) e^{i\mathbf{q}\cdot\mathbf{r}}. \tag{9}$$

This yields the following unsymmetrized strain field,

$$\frac{\partial u_\beta(\mathbf{r})}{\partial r_\lambda} = iU\left(\delta_{\beta z} q_\lambda - \delta_{\lambda z} q_\beta\right) e^{i\mathbf{q}\cdot\mathbf{r}} + U q_\beta q_\lambda z e^{i\mathbf{q}\cdot\mathbf{r}}. \tag{10}$$

The first term on the rhs describes the free *rotation* of the layer in response to a shear: the corresponding component of the elastic tensor vanishes, which results in the characteristic quadratic dispersion of the branch. By assuming propagation along $x$, the second term describes a symmetric strain of the type $\varepsilon_{xx} = Uq^2 z e^{iqx}$; this, in turn, yields a *transverse strain-gradient field* (i.e., a curvature $K$) of the type

$$K(x) = \varepsilon_{xx,z}(x) = Uq^2 e^{iqx} = -\frac{\partial^2}{\partial x^2} u_z(x), \tag{11}$$

consistent with Eq. (2) of the main text.

## 3 Microscopic response in curvilinear coordinates

Our theory rests on a powerful result of Ref. [3, 4], where the linear response of a microscopic field $f$ (either the charge density, the polarization or the electric field) to a slowly varying (on the scale of the lattice spacings) inhomogeneous strain field $\varepsilon_{\alpha\beta}(\mathbf{r})$ enjoys the following gradient expansion,

$$f^{(1)}(\mathbf{r}) = \varepsilon_{\alpha\beta}(\mathbf{r}) f^{\mathrm{U}}_{\alpha\beta}(\mathbf{r}) + \frac{\partial \varepsilon_{\alpha\beta}(\mathbf{r})}{\partial r_\gamma} f^{\mathrm{G}}_{\gamma,\alpha\beta}(\mathbf{r}) + \cdots. \tag{12}$$

Here $f^{(1)}$ stands for the total response to the deformation, while $f^{\mathrm{U}}_{\alpha\beta}(\mathbf{r})$ and $f^{\mathrm{G}}_{\gamma,\alpha\beta}(\mathbf{r})$ are cell-periodic functions describing the microscopic response to a uniform strain (U), and the additional contributions arising from the first gradient (G) of the strain. Note that $f$ stands for the curvilinear coordinate representation of the charge density, polarization and electric field, which are related to their Cartesian counterparts via the usual transformation rules for scalar densities, contravariant vector densities and covariant vectors, respectively. [3]

For a problem with cylindrical symmetry, it is useful to perform an in-plane average of all functions in Eq. (12), thus making the problem one-dimensional along $z$. Then, for a strain field of the type $\varepsilon_{\alpha\alpha}(z) = \lambda z$, corresponding to a macroscopically constant strain gradient $\varepsilon_{\alpha\alpha,z} = \lambda$, the out-of-plane component of the polarization and electric field read (at linear order in $\lambda$) as

$$P^{(1)}_z(z) = zP^{\mathrm{U}}_{z,\alpha\alpha}(z) + P^{\mathrm{G}}_{zz,\alpha\alpha}(z), \tag{13}$$

$$E^{(1)}_z(z) = zE^{\mathrm{U}}_{z,\alpha\alpha}(z) + E^{\mathrm{G}}_{zz,\alpha\alpha}(z). \tag{14}$$

By solving the curvilinear Poisson equation [Eq. (3) of the main text], within the linear regime of small deformations one obtains

$$E^{\mathrm{U}}_{z,\alpha\alpha}(z) = -\frac{1}{\epsilon_0} P^{\mathrm{U}}_{z,\alpha\alpha}(z) - E^{(0)}_z(z)(1 - 2\delta_{\alpha z}), \tag{15}$$

$$E^{\mathrm{G}}_{zz,\alpha\alpha}(z) = -\frac{1}{\epsilon_0} P^{\mathrm{G}}_{zz,\alpha\alpha}(z). \tag{16}$$

Here $E_z^{(0)}(z)$ is the electric field in the unperturbed ground state. (We assume that both $E^{\rm G}_{zz,\alpha\alpha}(z)$ and $P^{\rm G}_{zz,\alpha\alpha}(z)$ are defined and calculated while imposing open-circuit electrical boundary conditions along $\hat{z}$, consistent with the free-standing nature of the 2D film.) The total open-circuit voltage response to a strain-gradient deformation is then given by integrating the longitudinal electric field along $\hat{z}$,

$$\varphi = -\int_{-\infty}^{+\infty} dz \, \left[ z E^{\rm U}_{z,\alpha\alpha}(z) + E^{\rm G}_{zz,\alpha\alpha}(z) \right], \tag{17}$$

The second term in the square brackets yields the gradient, or "local flexoelectricity" contribution,

$$\varphi^{\rm G} \;=\; -\int_{-\infty}^{+\infty} dz \, E^{\rm G}_{zz,\alpha\alpha}(z). \tag{18}$$

The cell average of $P^{\rm G}_{zz,\alpha\alpha}(z)$ over a supercell containing the layer corresponds to the macroscopic 3D flexoelectric tensor, $\boldsymbol{\mu}$, of the slab/vacuum superlattice divided by the dielectric constant (recall that $\boldsymbol{\mu}$ is defined and calculated in short circuit); then, Eq. (18) immediately leads to Eq. (7) of the main text.

Regarding the remainder contributions, we combine Eq. (17) with Eq. (15) to obtain

$$\varphi^{\rm U} \;=\; \frac{1}{\epsilon_0} \int_{-\infty}^{+\infty} dz \, z P^{\rm U}_{z,\alpha\alpha}(z), \tag{19}$$

$$\varphi^{\rm M} \;=\; (1 - 2\delta_{\alpha z}) \int_{-\infty}^{+\infty} dz \, z E_z^{(0)}(z). \tag{20}$$

The second integral is easily calculated by parts, by observing that $\rho(z) = \epsilon_0 dE_z(z)/dz$,

$$\varphi^{\rm M} = -\frac{1 - 2\delta_{\alpha z}}{2\epsilon_0} \int_{-\infty}^{+\infty} dz \, z^2 \rho^{(0)}(z). \tag{21}$$

Note that $\rho^{(0)}(z)$ is the total ground-state charge density of the slab, including electrons and ions. The first integral goes by parts as well, but note the sign change that relates to the fact that the induced density is *minus* the divergence of $\mathbf{P}$, i.e. $\rho(z) = -dP(z)/dz$,

$$\varphi^{\rm U} = \frac{1}{2\epsilon_0} \int_{-\infty}^{+\infty} dz \, z^2 \rho^{\rm U}_{\alpha\alpha}(z). \tag{22}$$

Here $\rho^{\rm U}_{\alpha\alpha}(z)$ is the relaxed-ion charge-density response to a uniform strain $\varepsilon_{\alpha\alpha}$. After observing that $\delta_{\alpha z}$ vanishes for a transverse strain gradient, we readily recover Eq. (11) of the main text.

Interestingly, the present derivation is slightly more general in that it encompasses the case of a *longitudinal* strain-gradient deformation, obtained by setting $\alpha = z$ in the above equations. Because of the free-standing nature of the film, the static (fully-relaxed) response to a longitudinal strain gradient must vanish, regardless of the microscopic details of the material. While this result may be trivial from the physical point of view, it constitutes an excellent consistency check of our numerical implementation, and therefore we have used it systematically for all the materials that we have studied. We shall come back to this point in Section 4.5.

# 4 Clamped-ion and lattice-mediated coefficients

In this Section we proceed at decomposing the dipolar linear-response contributions (G and U) to the open-circuit voltage into clamped-ion (CI) and lattice-mediated (LM) contributions. Prior to that, we shall briefly recap the definition of the bulk flexoelectric tensor in the framework of linear-response theory. [2]

## 4.1 Bulk flexoelectric tensor in 3D

The bulk flexoelectric tensor can be written as a sum of electronic and lattice-mediated (LM) effects

$$\mu_{\alpha\lambda,\beta\gamma} = \underbrace{\mu^{\mathrm{el}}_{\alpha\lambda,\beta\gamma}}_{electronic} + \underbrace{\frac{1}{\Omega} Z^{(\alpha)}_{\kappa\rho} \left( \frac{\partial^2 E}{\partial u_{\kappa\rho} \partial u_{\kappa'\sigma}} \right)^{-1} C^{\kappa'}_{\sigma\lambda,\beta\gamma}}_{lattice-mediated} . \tag{23}$$

($\kappa$, $\kappa'$ run over atomic sublattices, other indices refer to Cartesian directions; summation over repeated indices is implied.) The second term is given by the product of the Born effective charge tensor, $Z^{(\alpha)}_{\kappa\rho}$, the *pseudoinverse* of the zone-center force-constant matrix (the latter is the second derivative of the total energy $E$ with respect to atomic displacements $u_{\kappa\sigma}$), and the flexoelectric force-response tensor, $C^{\kappa'}_{\sigma\lambda,\beta\gamma}$ (atomic forces induced by a strain gradient); $\Omega$ is the cell volume. Eq. (23) is in all respects analogous to the well-known formula for the static dielectric tensor, [5]

$$\epsilon_{\alpha\lambda} = \underbrace{\epsilon^{\mathrm{el}}_{\alpha\lambda}}_{electronic} + \underbrace{\frac{1}{\Omega} Z^{(\alpha)}_{\kappa\rho} \left( \frac{\partial^2 E}{\partial u_{\kappa\rho} \partial u_{\kappa'\sigma}} \right)^{-1} Z^{(\lambda)}_{\kappa'\sigma}}_{lattice-mediated} . \tag{24}$$

The electronic and force-response tensors of Eq. (23) can be further decomposed into a clamped-ion (indicated by a bar) and a remainder contribution,

$$\mu^{\mathrm{el}}_{\alpha\lambda,\beta\gamma} = \bar{\mu}_{\alpha\lambda,\beta\gamma} - P^{(1,\lambda)}_{\alpha,\kappa'\rho} \Gamma^{\kappa'}_{\rho\beta\gamma}, \tag{25a}$$

$$C^{\kappa}_{\alpha\lambda,\beta\gamma} = \bar{C}^{\kappa}_{\alpha\lambda,\beta\gamma} + \Phi^{(1,\lambda)}_{\kappa\alpha,\kappa'\rho} \Gamma^{\kappa'}_{\rho\beta\gamma}. \tag{25b}$$

Here $\Gamma^{\kappa'}_{\rho\beta\gamma}$ is piezoelectric internal-strain tensor, describing the atomic displacements induced by a uniform strain; $P^{(1,\lambda)}_{\alpha,\kappa'\rho}$ and $\Phi^{(1,\lambda)}_{\kappa\alpha,\kappa'\rho}$ refer, respectively, to the electronic polarization and atomic forces induced by a gradient of the mode $u_{\kappa'\rho}$ along the Cartesian direction $r_\lambda$. The clamped-ion terms in Eq. (25) describe the direct effect of a strain gradient on the electronic polarization (25a) and atomic forces (25b). The second terms in Eq. (25), mediated by the piezoelectric internal strain $\mathbf{\Gamma}$, reflect the indirect contribution of nonpolar lattice modes that couple linearly to a uniform strain.

The code implementation of the four "new" tensors in Eq. (25) relies on an analytic long-wave expansion [6] of the equations governing the linear response of the crystal to a phonon, electric field or "metric-wave" [7] perturbation. As of early 2020, a complete calculation of the bulk flexoelectric tensor including electronic and lattice-mediated effects can be carried out with the latest release of the ABINIT [8] package. The calculation is inexpensive on a modern workstation: It requires significantly less computational resources than a calculation of the phonon band structure.

### 4.2 Gradient contribution

Eq. (7) of the main text is written as the ratio of two relaxed-ion quantities (atomic units will be used throughout this derivation),

$$\varphi^{\rm G} = \frac{4\pi L}{\epsilon_{zz}} \mu_{zz,\alpha\alpha} = 4\pi L \frac{\mu^{\rm el}_{zz,\alpha\alpha} + \mu^{\rm LM}_{zz,\alpha\alpha}}{\epsilon^{\rm el}_{zz} + \epsilon^{\rm LM}_{zz}}, \tag{26}$$

respectively the macroscopic flexoelectric coefficient and the static dielectric constant of the supercell as defined in Eq. (23) and Eq. (24) above. It is not immediately clear how to recast the fraction as a sum of well-defined electronic and lattice-mediated terms. We shall proceed by writing

$$\varphi^{\rm G} = 4\pi L\, \hat{\mu}_{zz,\alpha\alpha}, \tag{27}$$

where $\hat{\mu}_{zz,\alpha\alpha}$ is constructed by imposing open-circuit (OC) boundary conditions along $z$ since the very beginning. More explicitly, one has the same formula Eq. (23)

$$\hat{\mu}_{zz,\alpha\alpha} = \underbrace{\hat{\mu}^{\rm el}_{zz,\alpha\alpha}}_{elec.} + \underbrace{\frac{1}{\Omega} \hat{Z}^{(z)}_{\kappa\beta}\, \hat{\Phi}^{-1}_{\kappa\beta\kappa'\gamma}\, \hat{C}^{\kappa'}_{\gamma z,\alpha\alpha}}_{latt.}, \tag{28}$$

in terms of the the electronic and lattice-mediated contributions ($\Phi^{-1}$ stands for the pseudoinverse), with the only difference that the symbols with a hat are defined here in OC.

To simplify the notation, from now on we shall adopt a bra/ket notation for the components of a given vector $v$ or operator $O$ over the atomic index and displacement direction,

$$\langle \kappa\alpha | v \rangle = v_{\kappa\alpha}, \qquad \langle \kappa\alpha | O | \kappa'\beta \rangle = O_{\kappa\alpha,\kappa'\beta}. \tag{29}$$

With this convention, Eq. (28) reads as

$$\hat{\mu}_{zz,\alpha\alpha} = \underbrace{\hat{\mu}^{\rm el}_{zz,\alpha\alpha}}_{elec.} + \underbrace{\frac{1}{\Omega} \langle \hat{Z}^{(z)} | \hat{\Phi}^{-1} | \hat{C}_{z,\alpha\alpha} \rangle}_{latt.}. \tag{30}$$

The electronic contribution and the force-response tensor, in turn, are defined analogously to Eq. (25) as

$$\hat{\mu}^{\rm el}_{zz,\alpha\alpha} = \hat{\bar{\mu}}_{zz,\alpha\alpha} - \frac{1}{2} \langle \hat{Q}^{(zz)} | \Gamma_{\alpha\alpha} \rangle, \tag{31a}$$

$$| \hat{C}_{z,\alpha\alpha} \rangle = | \hat{\bar{C}}_{z,\alpha\alpha} \rangle + \hat{\Phi}^{(1,z)} | \Gamma_{\alpha\alpha} \rangle. \tag{31b}$$

Note that the symmetric part of the $P^{(1,\lambda)}_{\alpha,\kappa\rho}$ tensor has the physical meaning of a quadrupolar response to an atomic displacement,

$$Q^{(\alpha\lambda)}_{\kappa\rho} = P^{(1,\lambda)}_{\alpha,\kappa\rho} + P^{(1,\alpha)}_{\lambda,\kappa\rho}, \tag{32}$$

where $\mathbf{Q}$ is the dynamical quadrupole tensor [6]. Note also the absence of the hat on $\Gamma^{\kappa}_{\beta\alpha\alpha}$ – $\mathbf{\Gamma}$ is unsensitive to the electrical boundary conditions since we have assumed inversion symmetry w.r.t. the $z = 0$ plane.

The conversion to OC of the purely electronic response functions is trivial, as it only entails a division by the out-of-plane component of the dielectric tensor,

$$\hat{\bar{\mu}}_{zz,\alpha\alpha} = \frac{\bar{\mu}_{zz,\alpha\alpha}}{\bar{\epsilon}_{zz}}, \tag{33}$$

$$|\hat{\bar{Z}}^{(z)}\rangle = \frac{1}{\bar{\epsilon}_{zz}}|\bar{Z}^{(z)}\rangle, \tag{34}$$

$$|\hat{\bar{Q}}^{(zz)}\rangle = \frac{1}{\bar{\epsilon}_{zz}}|\bar{Q}^{(zz)}\rangle. \tag{35}$$

The lattice-mediated response relies on several intermediate quantities. First, the pseudoinverse of the zone-center force-constant matrix is given by the Sherman-Morrison formula,

$$\hat{\Phi}^{-1} = \Phi^{-1} - \frac{4\pi}{\Omega}\frac{\Phi^{-1}|Z^{(z)}\rangle\langle Z^{(z)}|\Phi^{-1}}{\epsilon_{zz}}, \tag{36}$$

where

$$\epsilon_{zz} = \bar{\epsilon}_{zz} + \frac{4\pi}{\Omega}\langle Z^{(z)}|\Phi^{-1}|Z^{(z)}\rangle \tag{37}$$

is the static dielectric constant along the out-of-plane direction. Next, the clamped-ion force response transforms as

$$|\hat{\bar{C}}_{z,\alpha\alpha}\rangle = |\bar{C}_{z,\alpha\alpha}\rangle - \frac{4\pi\bar{\mu}_{zz,\alpha\alpha}}{\bar{\epsilon}_{zz}}|Z^{(z)}\rangle, \tag{38}$$

while the corresponding lattice-mediated part is governed by the nonanalytic behavior of the force-constant matrix at first order in $\mathbf{q}$ [see Supplemental Material of Ref. [9], Eq. (S.9)],

$$\hat{\Phi}^{(1,z)} = \Phi^{(1,z)} + \frac{4\pi}{\Omega}\frac{|Z^{(z)}\rangle\langle Q^{(zz)}| - |Q^{(zz)}\rangle\langle Z^{(z)}|}{2\bar{\epsilon}_{zz}}. \tag{39}$$

By combining Eq. (31) and Eqs. (38-39), we obtain the following result for the total force-response tensor in open circuit,

$$|\hat{C}_{z,\alpha\alpha}\rangle = |C_{z,\alpha\alpha}\rangle - \frac{4\pi\mu^{\rm el}_{zz,\alpha\alpha}}{\bar{\epsilon}_{zz}}|Z^{(z)}\rangle, \tag{40}$$

It is a tedious but otherwise straightforward exercise to verify that, with the above definitions, the following relation holds,

$$\hat{\mu}_{zz,\alpha\alpha} = \frac{\mu_{zz,\alpha\alpha}}{\epsilon_{zz}}. \tag{41}$$

## 4.3 Uniform strain contribution

The U term only contains one quantity that incorporates effects related to atomic relaxation, i.e. the charge-density response to a uniform strain. The relaxed-ion response, in particular, consists of a purely electronic and a lattice-mediated contribution,

$$\rho^{\rm U}_{\alpha\alpha}(z) = \bar{\rho}^{\rm U}_{\alpha\alpha}(z) + \Gamma^{\kappa}_{\beta\alpha\alpha}\rho^{\tau_{\kappa\beta}}(z), \tag{42}$$

where $\rho^{\tau_{\kappa\beta}}(z)$ is the charge-density response to an atomic displacement. We are left with the task of calculating

$$\int_{-\infty}^{+\infty} dz\, z^2 \rho^{\tau_{\kappa\beta}}(z). \tag{43}$$

To this end, we operate the following trick,

$$z^2 = (z-\tau_{\kappa z})^2 + 2(z-\tau_{\kappa z})\tau_{\kappa z} + \tau_{\kappa z}^2, \tag{44}$$

where $\tau_{\kappa z}$ is the unperturbed $z$ coordinate of atom $\kappa$. We obtain, for the relaxed-ion surface piezoelectricity contribution,

$$\varphi^{\rm U} = \bar{\varphi}^{\rm U} + \Delta\varphi^{(1)} + \Delta\varphi^{(2)}, \tag{45}$$

where the first term depends on the quadrupolar moment of the clamped-ion charge response to a strain,

$$\bar{\varphi}^{\rm U} = \frac{1}{2\epsilon_0}\int_{-\infty}^{+\infty} dz\, z^2 \bar{\rho}^{\rm U}_{\alpha\alpha}(z), \tag{46}$$

while the remainder two pieces contain the moments of the charge response to atomic displacements,

$$\Delta\varphi^{(1)} = \frac{1}{\epsilon_0}\Gamma^{\kappa}_{\beta\alpha\alpha}\tau_{\kappa z}\int_{-\infty}^{+\infty} dz\,(z-\tau_{\kappa z})\rho^{\tau_{\kappa\beta}}(z), \tag{47}$$

$$\Delta\varphi^{(2)} = \frac{1}{2\epsilon_0}\Gamma^{\kappa}_{\beta\alpha\alpha}\int_{-\infty}^{+\infty} dz\,(z-\tau_{\kappa z})^2\rho^{\tau_{\kappa\beta}}(z). \tag{48}$$

Now observe that

$$\int_{-\infty}^{+\infty} dz\,(z-\tau_{\kappa z})\,\rho^{\tau_{\kappa\beta}}(z) = \frac{Z^{(z)}_{\kappa\beta}}{S\bar{\epsilon}_{zz}}, \tag{49}$$

$$\int_{-\infty}^{+\infty} dz\,(z-\tau_{\kappa z})^2\rho^{\tau_{\kappa\beta}}(z) = \frac{Q^{(zz)}_{\kappa\beta}}{S\bar{\epsilon}_{zz}}, \tag{50}$$

where $S=\Omega/L$ is the cell surface. Finally, we have

$$\Delta\varphi^{(1)} = \frac{L}{\Omega\epsilon_0}\Gamma^{\kappa}_{\beta\alpha\alpha}\tau_{\kappa z}\,\hat{Z}^{(z)}_{\kappa\beta}, \tag{51}$$

$$\Delta\varphi^{(2)} = \frac{L}{2\Omega\epsilon_0}\Gamma^{\kappa}_{\beta\alpha\alpha}\,\hat{Q}^{(zz)}_{\kappa\beta}. \tag{52}$$

## 4.4 Total open-circuit voltage response

By combining the decompositions of $\varphi^{\rm U}$ and $\varphi^{\rm G}$ that we achieved in the above two sections, we obtain an elegant and compact result. In particular, the dipolar linear-response contribution enjoys an analogous expression as the bulk flexoelectric coefficient in OC [Eq. 23],

$$\mathcal{D}[\rho^{(1)}] = \underbrace{\mathcal{D}[\bar{\rho}^{(1)}]}_{elec.} + \underbrace{\frac{1}{S}\langle \hat{Z}^{(z)}|\hat{\Phi}^{-1}|\hat{\mathcal{C}}_{z,\alpha\alpha}\rangle}_{latt.}, \tag{53}$$

where the intermediate pieces are defined as,

$$\mathcal{D}[\bar{\rho}^{(1)}] = L\hat{\bar{\mu}}_{zz,\alpha\alpha} + \frac{\mathcal{Q}[\bar{\rho}^{\rm U}_{\alpha\alpha}]}{2\epsilon_0}, \tag{54a}$$

$$|\hat{\mathcal{C}}_{z,\alpha\alpha}\rangle = |\hat{\bar{C}}_{z,\alpha\alpha}\rangle + z|\Lambda_{\alpha\alpha}\rangle. \tag{54b}$$

Here $|\Lambda_{\alpha\alpha}\rangle$ is the piezoelectric force-response tensor, related to $\mathbf{\Gamma}$ by $|\mathbf{\Gamma}\rangle = \Phi^{-1}|\mathbf{\Lambda}\rangle$, and we have introduced the real-space position operator $z$, acting on the space of the bra/kets as

$$\langle\kappa\alpha|z|\kappa'\beta\rangle = \delta_{\kappa\kappa'}\delta_{\alpha\beta}\tau_{\kappa z}. \tag{55}$$

The full expression is

$$\hat{\mathcal{C}}^{\kappa}_{\beta z,\alpha\alpha} = \hat{\bar{C}}^{\kappa}_{\beta z,\alpha\alpha} + \Lambda^{\kappa}_{\beta\alpha\alpha}\tau_{\kappa z}. \tag{56}$$

By comparing these expressions with their 3D bulk counterparts, Eq. (30) and Eq. (31), one can identify two main differences: (i) averaging over the 2D cell surface $S$, rather than the 3D supercell volume, $\Omega$, is performed, consistent with the dimensionality of the problem; (ii) the terms that depend on the piezoelectric internal strain tensor $\mathbf{\Gamma}$ in Eq. (31) are replaced here by real-space moments along $z$ of the uniform-strain response functions $\bar{\rho}^{\rm U}_{\alpha\alpha}$ and $|\Lambda_{\alpha\alpha}\rangle$.

Remarkably, Eq. (54b) can be regarded as an application of the microscopic law Eq. (1) to the case of atomic forces induced by an inhomogeneous strain field – we could have anticipated it since the very beginning. It is not difficult to show that an analogous formula holds for the local atomic displacements,

$$\hat{\mathcal{L}}^{\kappa}_{\beta z,\alpha\alpha} = \hat{L}^{\kappa}_{\beta z,\alpha\alpha} + \Gamma^{\kappa}_{\beta\alpha\alpha}\tau_{\kappa z}, \tag{57}$$

where the flexoelectric internal-strain tensors are defined as $|\hat{\boldsymbol{\mathcal{L}}}\rangle = \hat{\Phi}^{-1}|\hat{\boldsymbol{\mathcal{C}}}\rangle$ and $|\hat{\mathbf{L}}\rangle = \hat{\Phi}^{-1}|\hat{\mathbf{C}}\rangle$ The derivation of the latter result rests on the definition of $\hat{\Phi}^{(1,z)}$: Since we are in open-circuit and the sample is finite along $z$, we can write $\hat{\Phi}^{(1,z)}$ as the first real-space moment of $\hat{\Phi}^{(0)}$ along $z$,

$$\hat{\Phi}^{(1,z)}_{\kappa\beta,\kappa'\gamma} = \hat{\Phi}^{(0)}_{\kappa\beta,\kappa'\gamma}(\tau_{\kappa z} - \tau_{\kappa' z}). \tag{58}$$

In practical calculations, we shall use the following procedure.

- First, we use the publicly available implementation of the bulk flexoelectric tensor in ABINIT to calculate the clamped-ion polarization ($\bar{\mu}_{zz,\alpha\alpha}$) and force-response ($|\bar{C}_{z,\alpha\alpha}\rangle$) tensors.

- Second, we convert these quantities to open-circuit boundary conditions according to the recipes of the earlier paragraphs,

$$\hat{\bar{\mu}}_{zz,\alpha\alpha} = \frac{\bar{\mu}_{zz,\alpha\alpha}}{\bar{\epsilon}_{zz}}, \tag{59}$$

$$|\hat{\bar{C}}_{z,\alpha\alpha}\rangle = |\bar{C}_{z,\alpha\alpha}\rangle - \frac{4\pi\bar{\mu}_{zz,\alpha\alpha}}{\bar{\epsilon}_{zz}}|Z^{(z)}\rangle, \tag{60}$$

| | $\varphi^{\mathrm{G}}$ | $\varphi^{\mathrm{M}}$ | $\varphi^{\mathrm{U}}$ | $\varphi$ |
|---|---|---|---|---|
| C | −3.8456 | −3.8456 | 7.6911 | 0.0000 |
| Si | −3.5106 | −3.5106 | 7.0213 | 0.0000 |
| P | −6.4059 | −6.4059 | 12.8118 | 0.0000 |
| BN | −3.5764 | −3.5744 | 7.1484 | −0.0024 |
| $MoS_2$ | −10.2987 | −10.2987 | 20.5975 | 0.0000 |
| $WSe_2$ | −12.0632 | −12.0630 | 24.1261 | −0.0001 |
| $SnS_2$ | −8.3634 | −8.3647 | 16.7271 | −0.0011 |

Table 1: Decomposition of the longitudinal $(zz, zz)$ flexovoltage coefficients according to the generalization of Eq. (5) described in Sec. 4.3.

- Finally, we incorporate the relevant uniform-strain contributions according to Eq. (54), thus obtaining the clamped-ion contribution to the dipole, and the total force response. The former, upon incorporation of the metric contribution, defines the CI flexovoltage. The latter defines the flexocoupling $f$ as

  $$f = \langle \kappa_{\mathrm{c}} z | \hat{\hat{C}}_{z,xx} \rangle, \tag{61}$$

  where $\kappa_{\mathrm{c}}$ refers to the cation sublattice.

### 4.5 The longitudinal case

To test the above formulas, it is very useful to consider the longitudinal case, where the results are already known analytically. We have, for the purely electronic response,

$$\varphi^{\mathrm{CI}} = \frac{1}{2\epsilon_0 S} \sum_{\kappa} \tau_{\kappa z}^2 \, \hat{Z}_{\kappa\beta}^{(z)}. \tag{62}$$

That is, the frozen-ion coefficient corresponds to the second moment of the longitudinal Born charges. Regarding lattice relaxation, the piezo internal-strain tensor is trivially written as

$$\Gamma_{\beta,zz}^{\kappa} = -\tau_{\kappa z} \, \delta_{\beta z}. \tag{63}$$

Next, the open-circuit flexo internal-strain tensor is given by

$$\hat{L}_{\beta z,zz}^{\kappa} = \left( \frac{1}{2} \tau_{\kappa z}^2 + K \right) \delta_{\beta z}, \tag{64}$$

where $K$ is an arbitrary constant independent of $\kappa$ that depends on the specific procedure that was used to construct the pseudoinverse – recall that the latter is not uniquely defined. $K$ in any case has no impact on the induced polarization because of the acoustic sum rule, so we can set it to zero. Finally, we have the corrected internal-strain tensor

$$\hat{\mathcal{L}}_{\beta z,zz}^{\kappa} = -\frac{1}{2} \tau_{\kappa z}^2 \, \delta_{\beta z}. \tag{65}$$

By putting all these results together, we find out that the purely electronic and the lattice-mediated part exactly cancel out, and the result vanishes as it should. Our numerical results (Table 1) are nicely consistent with this result, confirming the consistency of our implementation.

|  | $a$ (Å) | $b$ (Å) | $h$(Å) |
|---|---|---|---|
| C | 2.443 | 2.443 | 0.0000 |
| Si | 3.814 | 3.814 | 0.215 |
| P | 3.267 | 4.363 | 1.055 |
| BN | 2.473 | 2.473 | 0.0000 |
| $MoS_2$ | 3.121 | 3.121 | 1.553 |
| $WSe_2$ | 3.246 | 3.246 | 1.664 |
| $SnS_2$ | 3.618 | 3.618 | 1.468 |

Table 2: Equilibrium structural parameters for the unperturbed flat configuration of the materials considered in this work. $h$ corresponds to the thickness of the buckled materials.

# 5 Computational parameters

## 5.1 Primitive-cell linear-response calculations

Norm-conserving pseudopotentials are generated within Hamann's approach, [10] by using the "stringent" parameters of PseudoDojo, [11] but neglecting non-linear core corrections. We set a supercell size of $L = 30$ bohr (15.875 Å) and a plane-wave cutoff of 80 Ha; the Brillouin zone is sampled by a Γ-centered $12\times12\times2$ mesh except for graphene and silicene (a grid of $13\times13\times2$ points is used in the latter two cases); with respect to these parameters, the calculated flexovoltages are converged within a tolerance of 0.1% or better (see e.g. Fig. 3). Before performing the linear-response calculations, we optimize the atomic positions and cell parameters of the unperturbed systems to a stringent tolerance ($10^{-7}$ and $10^{-5}$ atomic units for residual stress and forces, respectively); the resulting structures (detailed in Tab. 2 and Fig. 2) are in excellent agreement with existing literature data (see e.g. Ref. [12] and references therein).

As a preliminary test of the method, we calculate the longitudinal flexovoltage coefficients, whose values are known analytically (see Sec. 4.5); we find (Table 1) excellent agreement with the expected results.

Note that most systems considered in this work (phosphorene is the only exception) are isotropic in plane, thus only one independent component of the flexovoltage needs to be calculated. For reference, we provide in Table 3 a decomposition of the CI part into the three contributions of Eq. (11) of the main text, namely the strain-gradient, uniform strain and geometric terms.

## 5.2 Direct nanotube calculations

BN nanotubes are constructed by folding a flat BN sheet via the transformation described in Sec. 2, with the tube axis oriented along the armchair direction. (These are known in the literature as "zigzag" BN nanotubes.) The resulting structures are then centered in an orthorhombic simulation cell of dimensions $L_y = \sqrt{3}a_0$ and $L_{x,z} = 4R$, with $R$ being the nanotube radius and $a_0$ the equilibrium lattice constant of the flat monolayer (see Table 2). We use the same pseudopotentials as in the linear-response calculations, a plane-wave cutoff of 60 Ha and a $1 \times 4 \times 1$ $k$-point mesh to sample the Brillouin zone. The flexovoltage is estimated as the voltage drop between the interior and exterior of the

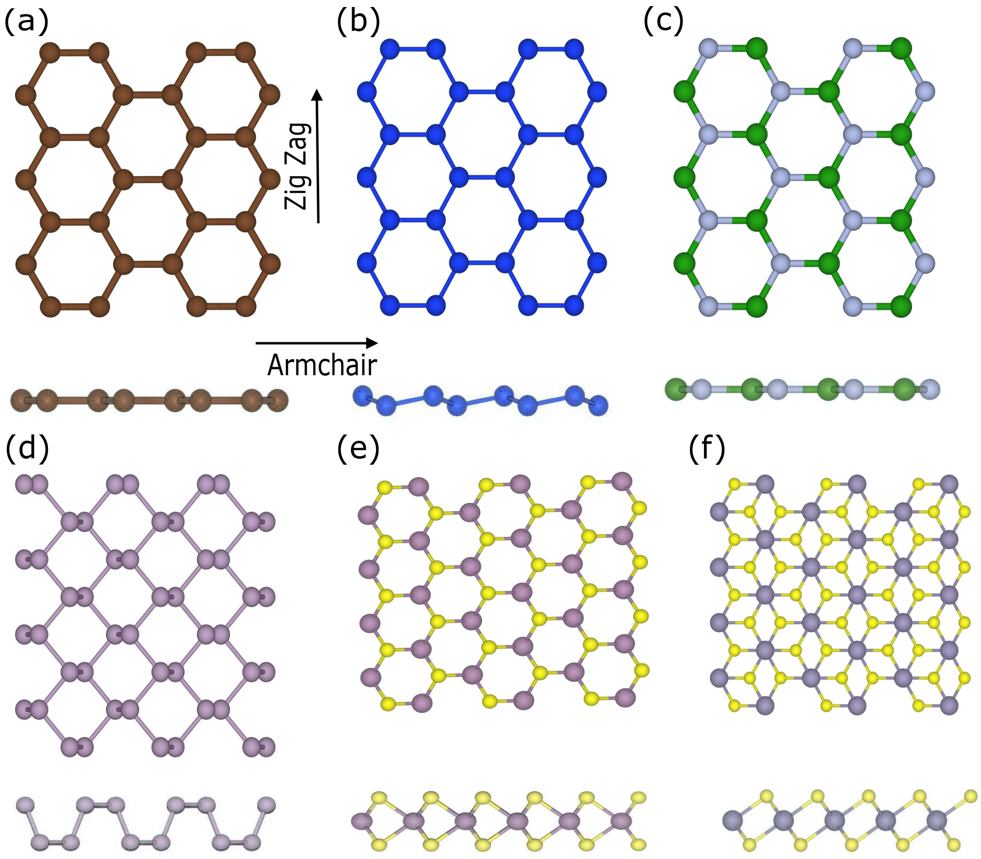


Figure 2: Top and side view of the crystal structures used in the calculations. (a) graphene, (b) silicene, (c) BN, (d) phosphorene, (e) $MoS_2$ and (f) $SnS_2$

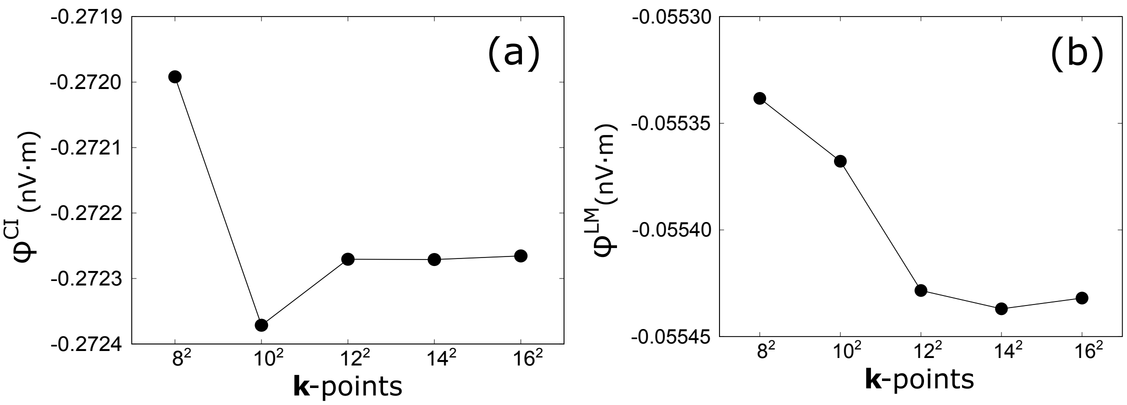


Figure 3: Convergence of clamped-ion (a) and lattice-mediated (b) $MoS_2$ flexovoltages as a function of the in-plane **k**-points mesh resolution. A plane-wave cutoff of 80 Hartree was employed in the calculations.

tube. In practice, after relaxing the electronic ground state at fixed atomic positions, we average the microscopic electrostatic potential along the tube axis, and extract the values at the center of the nanotube and at the fourfold-coordinated interstitial (equidistant point between four adjacent images).

# 6 Supplemental results

## 6.1 Analysis of the clamped-ion contribution

We report in Table 3 our results for the CI flexovoltage according to Eq. (11) of the main text. As we mentioned, the total flexovoltage results from the nearly complete cancellation of relatively large numbers. The sum of the first two columns of Table 3 yield the dipole moment of the first-order charge density response to the deformation, $\varphi^{\rm dip}$, which corresponds to the "radial polarization" as defined in Ref. [1]. $\varphi^{\rm dip}$ roughly coincides, within few percents, with the quadrupolar moment of the ground-state charge density divided by $2\epsilon_0$, hence the near cancellation with the metric term, $\varphi^{\rm M}$. This implies that an exceptional numerical accuracy is needed to compute the CI flexovoltage, $\varphi^{\rm CI} = \varphi^{\rm dip} + \varphi^{\rm M}$, highlighting the advantages of our linear-response formulation.

## 6.2 Analysis of the lattice-mediated contribution

For the compound materials that we have studied in this work, there is a single out-of-plane optical (ZO) mode that produces a net dipole. Such mode consists in the antiphase motion of the cation and anion sublattices, whereas either of them behaves as a rigid unit. This means that, in terms of these two degrees of freedom, the (open-circuit) force-constant matrix reduces to

$$\hat{\Phi}_{\kappa z \kappa' z} = a \begin{pmatrix} 1 & -1 \\ -1 & 1 \end{pmatrix}, \tag{66}$$

with $a$ a positive number, quantifying the strength of the restoring force. The reason is that $\hat{\Phi}_{\kappa z \kappa' z}$ must be a $2 \times 2$ matrix, and one of its eigenvalues must be zero (translational

| | $\frac{L\bar{\mu}_{zz,\alpha\alpha}}{\epsilon_0\bar{\epsilon}_{zz}}$ | $\frac{\mathcal{Q}[\bar{\rho}^{\rm U}_{\alpha\alpha}]}{2\epsilon_0}$ | $-\frac{\mathcal{Q}[\rho^{(0)}]}{2\epsilon_0}$ | $\varphi^{\rm CI}$ |
|---|---|---|---|---|
| C | −2.4658 | −1.4932 | 3.8456 | −0.1134 |
| Si | −2.3766 | −1.0755 | 3.5106 | +0.0585 |
| P (zigzag) | −5.2371 | −0.9364 | 6.4059 | +0.2323 |
| P (armchair) | −5.5274 | −0.8915 | 6.4059 | −0.0130 |
| BN | −2.2805 | −1.3320 | 3.5744 | −0.0381 |
| $MoS_2$ | −9.4562 | −1.1129 | 10.2987 | −0.2704 |
| $WSe_2$ | −11.4534 | −0.9254 | 12.0630 | −0.3158 |
| $SnS_2$ | −7.1838 | −0.9945 | 8.3647 | +0.1864 |

Table 3: Decomposition of the clamped-ion flexovoltage coefficient, $\varphi^{\rm CI}$, into the three contributions of Eq. (11) of the main text.

| | LDA | | | GGA | | |
|---|---|---|---|---|---|---|
| | $Z$ | $f$ | $a$ | $Z$ | $f$ | $a$ |
| BN | 0.2445 | −0.1131 | 0.1620 | 0.2444 | −0.1173 | 0.1515 |
| $MoS_2$ | −0.0854 | 0.3655 | 0.3323 | −0.0701 | 0.2980 | 0.3056 |
| $WSe_2$ | −0.0992 | 0.4222 | 0.3134 | −0.0805 | 0.2871 | 0.2876 |
| $SnS_2$ | 0.3429 | 0.2291 | 0.2030 | 0.3557 | 0.1794 | 0.1854 |

Table 4: Dynamical charge ($Z$), flexocoupling coefficient ($f$) and ZO mode stiffness ($a$) for selected materials (atomic units) calculated with LDA and GGA. The sign of the polar mode eigenvector is set in such a way that the cation moves outwards.

invariance), the other positive; this leaves only one free parameter.

To calculate $\varphi^{\rm LM}$ we need the pseudoinverse of this. To this end, we first calculate eigenvalues and eigenvectors,

$$\lambda_1 = 0, \qquad v_1 = \frac{1}{\sqrt{2}}(1,1), \tag{67}$$

$$\lambda_2 = 2a, \qquad v_2 = \frac{1}{\sqrt{2}}(1,-1). \tag{68}$$

We can write then

$$\hat{\Phi}^{-1}_{\kappa\kappa'} = \frac{1}{4a}\begin{pmatrix} 1 & -1 \\ -1 & 1 \end{pmatrix}, \tag{69}$$

The longitudinal dynamical charges,

$$\hat{Z}^{(z)}_{\kappa z} = (Z, -Z), \tag{70}$$

and the (OC) flexoelectric force response,

$$\hat{\mathcal{C}}^{\kappa}_{zz,\alpha\alpha} = (f, -f). \tag{71}$$

are also governed by a single parameter each. (The sublattice sum of the dynamical charges vanishes due to the acoustic sum rule; moreover, since the crystal is a 2D layer suspended in vacuum, the sum of the flexoforces must vanish.) Thus, the LM flexovoltage is given by

$$\varphi^{\rm LM} = \frac{1}{\epsilon_0 S}\frac{Zf}{4a}\begin{pmatrix} 1 & -1 \end{pmatrix}\begin{pmatrix} 1 & -1 \\ -1 & 1 \end{pmatrix}\begin{pmatrix} 1 \\ -1 \end{pmatrix} = \frac{1}{\epsilon_0 S}\frac{Zf}{a}, \tag{72}$$

Thus, the lattice-mediated effect acquires the intuitive physical meaning of a geometric field distorting the lattice along the ZO mode coordinate by an amount $u$ that is proportional to the coupling $f$ and inversely proportional to the mode stiffness, $a$. Such displacement, in turn, produces a dipole per unit area that goes like $u \times Z$. Note that the mode stiffness $a$ relates to the ZO phonon frequency $\omega$ via $a = m\omega^2$, where $m$ is the reduced mass of the two-body system.

To help understand the lattice-mediated part, we have calculated the physical constants entering Eq.(72). From the results reported in Table 4, one can see that the flexocoupling

| | $\varphi^{\mathrm{CI}}$ | $\varphi^{\mathrm{LM}}$ | $\varphi^{\mathrm{tot}}$ |
|---|---|---|---|
| C | −0.1245 | 0.0000 | −0.1245 |
| Si | 0.0297 | 0.0000 | 0.0297 |
| P (zigzag) | 0.2495 | −0.0105 | 0.2390 |
| P (armchair) | 0.0372 | −0.0311 | 0.0062 |
| BN | −0.0502 | −0.1760 | −0.2262 |
| $MoS_2$ | −0.3301 | −0.0395 | −0.3696 |
| $WSe_2$ | −0.3739 | −0.0531 | −0.4269 |
| $SnS_2$ | 0.1763 | 0.1467 | 0.3229 |

Table 5: GGA values of the clamped-ion (CI), lattice-mediated (LM) and total flexovoltage (nV·m) coefficients of the 2D crystals studied in this work.

strength is roughly proportional (in absolute value) to the mode stiffness; this means that in these materials the magnitude of the LM response is largely determined by the dipolar strength of the ZO mode, $Z$. The sign of the effect, as in the CI response, varies across the tested set. Bending tends to produce an outward force on the cation, except in BN; however, in some TMDs the anomalous sign [13] of the dynamical charges results in a negative LM response in spite of $f$ being positive.

### 6.3 Generalized-gradient approximation

In order to check whether the treatment of the exchange and correlation energy has a strong impact on our results, we have recalculated the flexovoltages of Table I of the main text by using the PBE [14] formulation of the generalized-gradient approximation (GGA). To perform these calculations, we had to extend our computational methodologies to allow for the treatment of generalized-gradient (GGA) functionals first. Details of the implementation and tests will be published elsewhere; a flavor of the technical challenges that GGA presents in linear-response problems involving strain can be found in Ref. [15]. Our results, reported in Table 5, indicate that the deviations from the LDA values are relatively minor, and amount to about 10 % in most cases. Larger relative changes only occur in coefficients that were already small in the first place; examples are silicene, P (armchair), and the CI coefficient of BN.

### 6.4 Comparison to the literature

Most numerical calculations reported in the literature on flexoelectricity of 2D materials have adopted a 3D volume-averaged definition of the flexoelectric coefficients. The general approach to estimate the latter has been to explicitly bending a finite ribbon [16, 17, 18, 19] or an extended 2D sheet, [20] relaxing the atomic positions in the deformed structure and estimating the induced polarization ($P_z$) as the out-of-plane dipole moment. A flexoelectric coefficient $\mu$, in units of charge per unit length, is finally extracted from the slope of the $P_z$ vs. $1/R$ adjust ($R$ being the curvature radius).

We recall that such a definition of $\mu$ is inappropriate for 2D materials where the layer thickness $t$, and therefore the cell volume, is an ill-defined quantity. In Table 6.4 we convert,

| | $t$ (Å) | $\varphi$ (nV·m) | $\mu$ (pC/m) |
|---|---|---|---|
| Si | 3.18 | 0.0585 | 1.6273 ($7.28^a$) |
| C | 3.34 | −0.1134 | −3.0062 ($2.86^a$, $0.4^d$) |
| BN | 3.85 | −0.2009 | −4.6202 ($0.26^a$) |
| P (zigzag) | 5.61 | 0.2170 | 3.4245 ($46^b$) |
| P (armchair) | 5.61 | −0.0591 | −0.9327 ($84^b$) |
| $SnS_2$ | 6.98 | 0.3592 | 4.5577 |
| $MoS_2$ | 7.44 | −0.3269 | −3.8906 ($31.94^a$, $-1.82^c$) |
| $WSe_2$ | 7.53 | −0.3899 | −4.5819 ($-0.78^c$) |

Table 6: Interlayer spacing in the bulk (extracted from Ref. [21]), total flexovoltage and volume-averaged flexoelectric coefficient of the 2D crystals studied in this work. Data between round brackets in the third column has been extracted from the literature: $^a$ Ref. [16],$^b$ Ref. [18], $^c$ Ref. [20], $^d$ Ref. [17]

for the sake of comparison, the $\mu^{2D}$ coefficients obtained in this work to the $\mu$ units as $\mu = \mu^{2D}/t$ and contrast them with the reported values. We used the interlayer spacing in the corresponding bulk structures as an estimate of the monolayer thickness $t$. The data shown in the third column of the table indicate a large dispersion, in both sign and magnitude, when comparing our results with the values found in the literature. The latter also markedly differ among themselves, as can be observed, e.g., in the coefficients reported for graphene and $MoS_2$ .

# 7 An illustrative toy model: Xe monolayer

As a further consistency check of the theory developed so far, we consider a hexagonal Xe monolayer as shown in Fig.(4). This system is only weakly bonded, and becomes a trivial 2D lattice of noninteracting spherical atoms in the limit of a large lattice parameter. In such a limit, the flexoelectric response must vanish, following the arguments of Ref. [3] and Ref. [4]. Thus, it provides a testcase where we can benchmark our computational method against an analytically known exact result. In particular, we shall demonstrate the essential role of the metric term to extract sensible physical conclusions.

Fig. 5 summarizes the results for $\varphi^{\rm dip}$, $\varphi^{\rm M}$ and $\varphi^{\rm tot} = \varphi^{\rm dip} + \varphi^{\rm M}$, as a function of the in-plane lattice parameter; note that $\varphi^{\rm dip}$ consists in the dipole moment of the first-order charge density, and thus coincides with "radial polarization" as defined in Ref. [1].

Clearly, $\varphi^{\rm dip}$ and $\varphi^{\rm M}$ are large in absolute value and opposite in sign. As a result, the "total" flexovoltage $\varphi^{\rm (tot)}$ is always negligibly small, and vanishes exponentially (inset of fig.5) in the limit of large $a_0$, consistent with the expectations. [3] Upon closer inspection, we find that the large absolute values of $\varphi^{\rm dip,M}$ essentially coincide with the quadrupolar moment of $\phi^{\rm Xe}(\mathbf{r})$, i.e., the spherical charge density of an isolated Xe atom, divided by the cell surface ($S$),

$$\varphi^{\rm dip,M} \simeq \pm \frac{Q}{2S\epsilon_0}, \qquad Q = \int d^3r x^2 \phi^{\rm Xe}(\mathbf{r}). \tag{73}$$

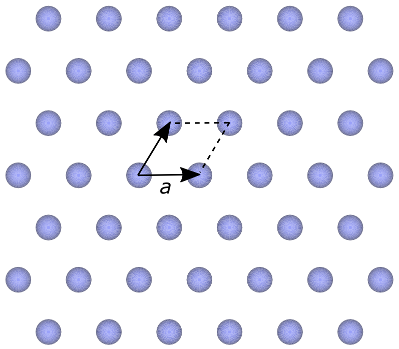


Figure 4: Crystal structure of the hexagonal Xe monolayer discussed in the text.

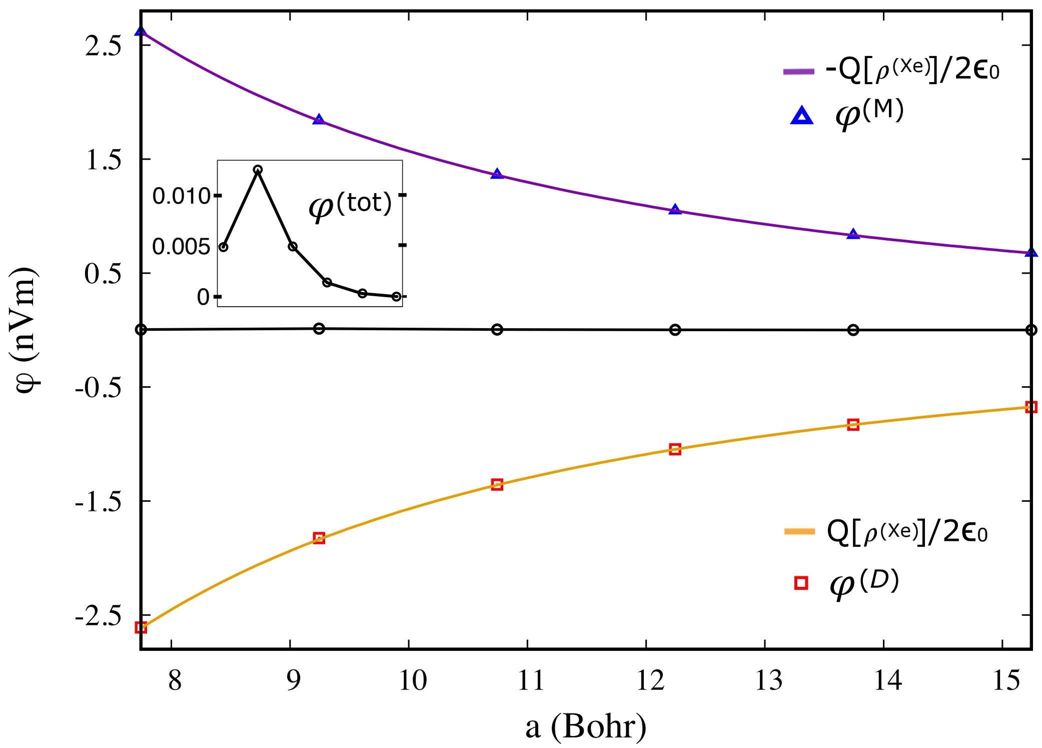


Figure 5: Computed values for $\varphi^{(\mathrm{M})}$, $\varphi^{(\mathrm{D})}$, $\varphi^{(\mathrm{tot})}$ (nVm) and the analytical curves given by $\left(\mp\mathcal{Q}[\rho^{(\mathrm{Xe})}]/2\varepsilon_0\right)$, as a function of the of the increasing in-plane lattice constant. $\mathcal{Q}[\rho^{(\mathrm{Xe})}]$ is the quadrupolar moment of the isolated atom divided by the unit cell surface $S \propto a^2$. The inset shows the computed values of the “total” flexovoltage, otherwise indistinguishable from zero, being three orders of magnitude smaller then the dipolar and metric terms reported in the figure.

To show this, we calculate $Q$ once and for all as the large-$a_0$ limit of $-2S\epsilon_0\varphi^{\rm M}$, and we plot $\pm Q/2S\epsilon_0$ as continuous curves in Fig. 5; the matching with the first-principles data is excellent.

To rationalize this result, it is useful to work out the analytical solution to this problem in the noninteracting (large $a_0$) limit. To understand why the flexovoltage must vanish it is most convenient to work in the Cartesian frame. Then, the transverse deformation of Sec. 2.1 can be described as a displacement of each atom $l$ to a distorted location,

$$\mathbf{R}_l = \mathbf{f}(\mathbf{R}_l^{(0)}), \tag{74}$$

where $\mathbf{R}_l^{(0)}$ span the unperturbed 2D Bravais lattice and $\mathbf{f}$ is the mapping of Eq. (1b). The fact that the atoms "do not see each other" implies that the total (electronic and ionic) charge density of the system in both the unperturbed and perturbed configurations is simply a superposition of the spherical atomic densities,

$$\rho^{(0)}(\mathbf{r}) = \sum_l \phi^{\rm Xe}(\mathbf{r}-\mathbf{R}_l^{(0)}), \qquad \rho(\mathbf{r}) = \sum_l \phi^{\rm Xe}(\mathbf{r}-\mathbf{R}_l). \tag{75}$$

This observation explains why the flexovoltage vanishes: each atom remains perfectly spherical, and hence cannot generate a long-range potential no matter how much the "layer" is deformed (i.e., how far the constituent atoms are moved around).

To understand the result of Fig. 5 for the individual (dipolar and metric) contributions to the total flexovoltage, we need to solve the same problem in the curvilinear coordinate system that corresponds to the nanotube geometry described in Sec. 2. $\rho(\mathbf{r})$ transforms as a scalar density, which yields the following relation between its curvilinear and Cartesian representation, [4]

$$\rho^{\rm Cart}(\mathbf{r}') = h^{-1}\hat{\rho}(\mathbf{r}), \tag{76}$$

where $h$ is the Jacobian determinant of the coordinate transformation. This is very convenient, as in the curvilinear frame the atoms do not move from their original location, and

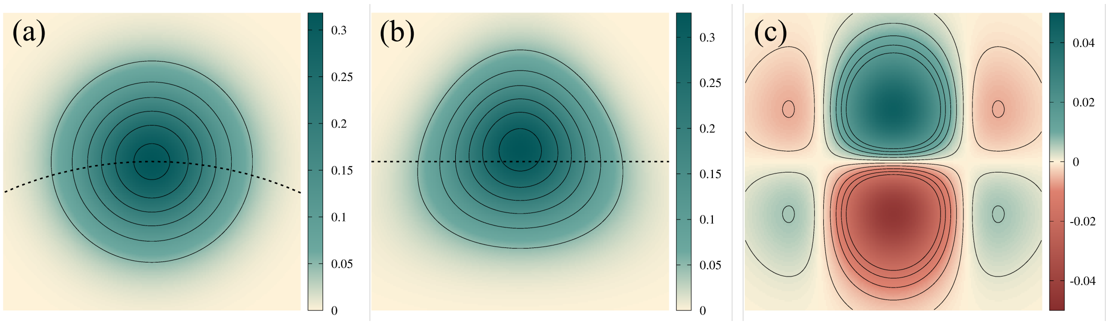


Figure 6: Impact of curvature on the charge density of a rigid spherical object. For illustration purposes, we use a Gaussian function centered in the origin of the type $\phi(\mathbf{r}) = \frac{1}{\pi\sigma^2}e^{-r^2/\sigma^2}$. (a): Cartesian representation; the dashed curve indicates the curved layer plane. (b): curvilinear $\hat{\rho}(\mathbf{r})$ as defined in Eq. (76); the deformation of the original Gaussian is clear. (c): first-order variation of $\hat{\rho}(\mathbf{r})$ as given by Eq. (80).

the charge density $\hat{\rho}(\mathbf{r})$ retains the full translational periodicity of the undeformed 2D crystal. This, however, also implies that an atom that is spherically symmetric in the Cartesian frame is generally no longer spherical in the curvilinear system. In other words, for the noninteracting atoms to retain their spherical ground state in the deformed configuration, *the curvilinear charge density must respond to the deformation in order to compensate for the consequences of the coordinate transformation.* This results in an apparent transfer of charge, $\Delta\hat{\rho}$, that does not originate from the local chemistry (and indeed no chemistry is going on in this system), but is simply a mathematical by-product of the coordinate transformation: it can be calculated analytically by inverting Eq. (76).

Within the regime of small deformations, $\Delta\hat{\rho}(\mathbf{r})$ can be written as [4]

$$\Delta\hat{\rho}(\mathbf{r}) = z\rho^{\mathrm{U}}_{xx}(\mathbf{r}) + \rho^{\mathrm{G}}_{xx,z}(\mathbf{r}), \tag{77}$$

where the two functions on the rhs are the microscopic density response to a uniform (U) strain and a strain gradient (G). [2, 3] The latter functions are easy to derive by using Eqs.(90–91) of Ref. [4], in conjunction with Eq. (75) of Ref. [2], and by observing that the charge-density response to the displacement of an isolated atom is given by translational invariance as

$$\frac{\partial\rho(\mathbf{r})}{\partial R_{l\beta}} = \phi^{\mathrm{Xe}}_{\beta}(\mathbf{r}-\mathbf{R}_l), \qquad \phi_\beta(\mathbf{r}) = -\frac{\partial}{\partial r_\beta}\phi^{\mathrm{Xe}}(\mathbf{r}). \tag{78}$$

We find

$$\rho^{\mathrm{U}}_{xx} = \rho^{(0)}(\mathbf{r}) - \sum_l (x - X_l)\phi_x(\mathbf{r}-\mathbf{R}_l), \tag{79a}$$

$$\rho^{\mathrm{G}}_{xx,z} = \sum_l (x-X_l)(z-Z_l)\phi_x(\mathbf{r}-\mathbf{R}_l) - \frac{1}{2}(x-X_l)^2\phi_z(\mathbf{r}-\mathbf{R}_l). \tag{79b}$$

After few steps of straightforward algebra, we obtain (an illustration is provided in Fig. 6)

$$\Delta\hat{\rho}(\mathbf{r}) = \sum_\kappa \xi(\mathbf{r}-\mathbf{R}_\kappa), \qquad \xi(\mathbf{r}) = z\phi(\mathbf{r}) + \frac{x^2}{2}\frac{\partial\phi(\mathbf{r})}{\partial z}. \tag{80}$$

Since $\Delta\hat{\rho}(\mathbf{r})$ retains in-plane periodicity, $\mathcal{D}[\Delta\hat{\rho}]$ reduces to the dipolar moment of $\xi(\mathbf{r})$,

$$\begin{aligned}\mathcal{D}[\Delta\hat{\rho}] =& \frac{1}{S}\int d^3r\, z\xi(\mathbf{r}) \\ =& \frac{1}{S}\int d^3r \left[z^2\phi(\mathbf{r}) + \frac{x^2}{2}z\frac{\partial\phi(\mathbf{r})}{\partial z}\right] \\ =& \frac{Q}{\epsilon_0 S} - \frac{Q}{2\epsilon_0 S} = \frac{Q}{2\epsilon_0 S},\end{aligned} \tag{81}$$

thus proving por point. (We used the spherical symmetry of $\phi(\mathbf{r})$ and an integration by parts along $x$.)

This result clearly illustrates that $\varphi^{\mathrm{dip}}$ does not correspond to a meaningful physical property of the system: it contains spurious contributions that are mathematical artefacts of the coordinate transformation, and the "metric" term is essential to remove such unphysical terms from $\varphi^{\mathrm{tot}}$.

# 8 Coupling between out-of-plane electric fields and flexural phonons

In this Section we shall discuss the direct and converse flexoelectric effect within a more rigorous treatment of the electrostatics in 2D.

## 8.1 Macroscopic electric fields in 2D

A flexural phonon produces an external charge perturbation of the form

$$\rho^{\text{ext}}(\mathbf{r}) = e^{i\mathbf{q}\cdot\mathbf{r}}\rho^{\mathbf{q}}(z), \tag{82}$$

where $\rho^{\mathbf{q}}(z)$ is the planar average of the cell-periodic part. We shall calculate the electrostatic potential at some far-away point from the layer. We shall use the Coulomb kernel as defined in Ref. [22],

$$\nu(\mathbf{q}, z - z') = \frac{2\pi}{q} e^{-q|z-z'|}, \tag{83}$$

The potential can then be written as a convolution in real space,

$$V^{\mathbf{q}}(z) = \int dz'\, \nu(\mathbf{q}, z - z')\rho^{\mathbf{q}}(z'). \tag{84}$$

If we consider a point in the $z > 0$ plane that is located far enough from the layer that the perturbed density vanishes, the potential is simply given by

$$V^{\mathbf{q}}(z) = \frac{2\pi}{q} \int dz'\, e^{-q(z-z')}\rho^{\mathbf{q}}(z') = \frac{2\pi}{q} e^{-qz} \int dz'\, e^{qz'}\rho^{\mathbf{q}}(z'). \tag{85}$$

For the $z < 0$ plane we have, similarly,

$$V^{\mathbf{q}}(z) = \frac{2\pi}{q} \int dz'\, e^{q(z-z')}\rho^{\mathbf{q}}(z') = \frac{2\pi}{q} e^{qz} \int dz'\, e^{-qz'}\rho^{\mathbf{q}}(z'). \tag{86}$$

Now observe that

$$e^{qz} = \cosh(qz) + \sinh(qz), \qquad e^{-qz} = \cosh(qz) - \sinh(qz). \tag{87}$$

It is then convenient to introduce the following two integrals,

$$\rho^{\parallel}(\mathbf{q}) = \int dz\, \rho^{\mathbf{q}}(z)\cosh(qz), \tag{88}$$

$$\rho^{\perp}(\mathbf{q}) = \int dz\, \rho^{\mathbf{q}}(z)\sinh(qz). \tag{89}$$

Then, we obtain

$$V^{\mathbf{q}}(z > 0) = \frac{2\pi}{q} e^{-q|z|} \left[\rho^{\parallel}(\mathbf{q}) + \rho^{\perp}(\mathbf{q})\right], \tag{90}$$

$$V^{\mathbf{q}}(z < 0) = \frac{2\pi}{q} e^{-q|z|} \left[\rho^{\parallel}(\mathbf{q}) - \rho^{\perp}(\mathbf{q})\right]. \tag{91}$$

This provides the formal link between the stray fields in the vacuum region and an arbitrary external charge that is modulated within the layer plane at some wave vector $\mathbf{q}$. Consistent with the arguments of Ref. [22], the information about the macroscopic electrostatic potentials (i.e. the fields in the vacuum region where the charge density perturbation vanishes) is exactly contained in the two hyperbolic integrals $\rho^{\parallel}(\mathbf{q})$ and $\rho^{\perp}(\mathbf{q})$.

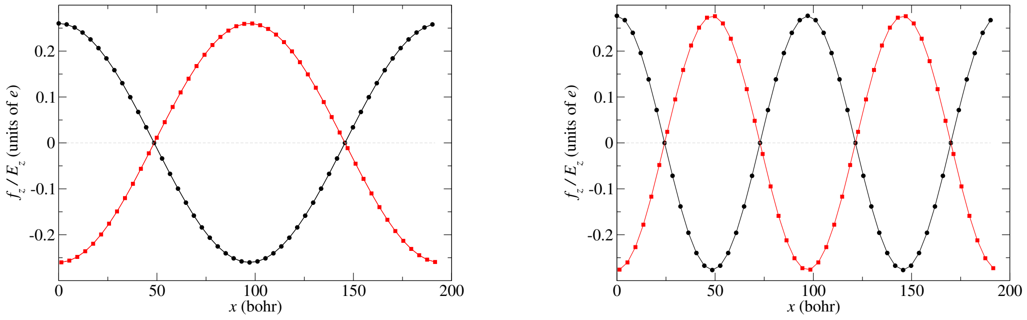


Figure 7: Atomic forces induced by a spatially modulated transverse electric field on a BN monolayer in its unperturbed equilibrium structure. Modulation periods of 24 (left) and 12 (right) cells are shown. Black circles and red squares refer to B and N atoms, respectively. Solid curves are fits to the data (see text).

### 8.2 Flexovoltage

To connect with the theory developed in the main text, we need to extract the potential discontinuity near $z = 0$ for the mirror-odd (sinh) component of the field,

$$V^{\perp}(\mathbf{q}) = V^{\mathbf{q}}(+\epsilon) - V^{\mathbf{q}}(-\epsilon) = \frac{4\pi}{q}\rho^{\perp}(\mathbf{q}). \tag{92}$$

Based on the arguments of Sec. 2.2, at the leading order in $q$ we must have $V^{\perp}(\mathbf{q}) = 4\pi q^2 \mu^{\text{2D}} = q^2\varphi$; this implies

$$\rho^{\perp}(\mathbf{q})/q = q^2\mu^{\text{2D}} + \cdots . \tag{93}$$

This formula is important, because it expresses the out-of-plane flexoelectric coefficient of the layer as a second derivative of the total energy with respect to two well-defined perturbations: (i) a flexural phonon distortion at some wavevector $\mathbf{q}$, and (ii) a modulated electric field, described by an externally applied scalar potential of the type

$$V^{\text{ext}}(\mathbf{r}) = -\mathcal{E}_z \frac{\sinh(qz)}{q}\cos(\mathbf{q}\cdot\mathbf{r}). \tag{94}$$

This observation guarantees the thermodynamic equivalence between the direct and converse flexoelectric effect, as we shall see in the following subsection. Right on the $z = 0$ plane (i.e., in the strict 2D limit), Eq. (94) corresponds to a pure transverse field, modulated by a complex phase. In a neighborhood of the layer, the hyperbolic sine function constitutes the correct [22] generalization of the latter to the quasi-2D case. As a matter of fact, one can show that *any* statically applied potential with mirror-odd symmetry can be expanded on a basis of $\sinh(qz)$ functions times an in-plane phase. This implies that our considerations hold, in full generality, for an arbitrary inhomogeneous field applied out-of-plane.

### 8.3 Converse flexoelectric effect in 2D

As a numerical demonstration of the above results, we have performed an explicit numerical test by applying the external potential of Eq. (94) to a suspended monolayer of BN within

| Period (cells) | $Z_{\mathrm{B}}$ | $Z_{\mathrm{N}}$ | $\sum_{\kappa} Z_{\kappa}$ | $\bar{\mu}^{\mathrm{2D}}$ |
|---|---|---|---|---|
| 12 | 0.276832 | −0.277014 | −0.000182 | −0.00230 |
| 24 | 0.260273 | −0.260315 | −0.000042 | −0.00212 |

Table 7: Explicit calculation of the converse flexoelectric effect. $Z_\kappa$ are the fitted atomic forces in response to the modulated field; $\bar{\mu}^{\mathrm{2D}}$ is the estimated clamped-ion flexoelectric coefficient calculated according to Eq. (96). All values are in units of electron charge.

free electrical boundary conditions. [We have used a $24\sqrt{3} \times 1$ supercell, with similar computational parameters to those that we used in the linear-response calculations reported in the main text; we have tested two values of $q = 2\pi/(N\sqrt{3}a_0)$, with $N = 12, 24$.] After relaxing the electronic ground state in the external field at fixed atomic positions, we have extracted the out-of-plane atomic forces; their values divided by the field amplitude (we use $\mathcal{E}_z = 10^{-4}$ atomic units) are shown in Fig. 7.

The forces display an essentially perfect match with a cosine function, whose amplitude is close to the out-of-plane Born charge of the sublattice,

$$f^l_\kappa = Z_\kappa(\mathbf{q}) \cos(\mathbf{q} \cdot \mathbf{R}_{l\kappa}). \tag{95}$$

The values of the fit, reported in Table 7, show that the forces on the two sublattices do not cancels exactly; their sum, according to the above arguments, are related to the clamped-ion flexoelectric coefficient, $\bar{\mu}^{\mathrm{2D}}$ by

$$\frac{1}{q^2 S} \sum_\kappa f_\kappa \simeq \bar{\mu}^{\mathrm{2D}}. \tag{96}$$

The resulting values are in excellent agreement with the direct coupling coefficient calculated via linear-response (see Table I of the main text), $\bar{\mu}^{\mathrm{2D}} = -0.002105e$, demonstrating the internal consistency of our arguments. Note the relative smallness of the flexoelectric coupling [an $O(q^2)$ effect] compared to the force on the optical "ZO" phonon of the monolayer (given by the *difference* $Z_{\mathrm{B}} - Z_{\mathrm{N}}$). The restoring force of the flexural phonon, however, goes like $O(q^4)$, which means that the resulting distortions can be very large in the long-wavelength limit, as we shall see in the next subsection.

## 8.4 Continuum modeling of PFM experiments

Incorporation of Eq.(13) of the main text into the model of Ref. [23] leads to the following continuum energy functional,

$$E(u, \mathcal{E}) = \frac{g}{2} u^2 + \frac{B}{2} \left(\nabla^2 u\right)^2 + \mu^{\mathrm{2D}} \mathcal{E} \nabla^2 u. \tag{97}$$

Here $u(x, y)$ is the vertical displacement of the layer, $\mathcal{E}(x, y)$ is the out-of-plane field, $\nabla^2$ is the in-plane Laplacian operator, $g$ describes the coupling to the substrate (the latter is assumed to be clamped for simplicity), and $B$ is the bending modulus. Of the three parameters appearing in Eq. (97), $B$ and $\mu^{\mathrm{2D}}$ are well-defined *intrinsic* properties of the crystal; $g$ obviously depends on the specifics of the experimental setup.

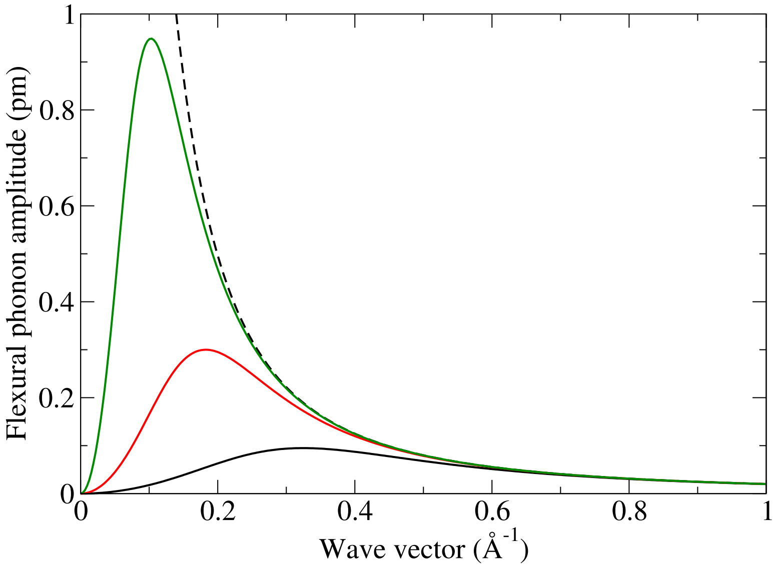


Figure 8: Amplitude of the flexural phonon response to an externally applied transverse electric field of 1 GV/m, modulated at a given in-plane wavevector $q$. Results for $g = 10^{-1}$ eV/Å$^4$ (black), $g = 10^{-2}$ eV/Å$^4$ (red), $g = 10^{-3}$ eV/Å$^4$ (green) and the free-standing layer (dashed) are shown.

As an example, in Fig. 8 we show a reciprocal-space analysis of the vertical displacement amplitude, which we performed by assuming a cosine-like form for both functions $\mathcal{E}$ and $u$. After substituting $f(x) = f \cos(\mathbf{q} \cdot \mathbf{r})$ $[f = \mathcal{E}, u]$ in Eq. (97) we obtain

$$E(u, \mathcal{E}) = \frac{g + Bq^4}{2} u^2 - \mu^{2\mathrm{D}} \mathcal{E} q^2 u, \quad \rightarrow \quad u = \frac{\mu^{2\mathrm{D}} \mathcal{E} q^2}{g + Bq^4}, \tag{98}$$

where the second equality stems from the stationary condition on $E$. By using the physical parameters of $MoS_2$, $\mu^{2\mathrm{D}} = -0.018e$ and $B = 9$ eV [24], and four different choices for the substrate interaction parameter, $g$. (The largest value of $g$=0.1 eV/Å$^4$ roughly corresponds to the interlayer coupling in bulk $MoS_2$; depending on the substrate and deposition technique, the interaction may be one or two orders of magnitude weaker.) The free-standing solution diverges as $q^{-2}$ (a uniform field induces a curvature of $K = \mu^{2\mathrm{D}} \mathcal{E}/B$ in such a limit), while in presence of interaction the response peaks at some wavevector $q$ and vanishes in the limit of a uniform field (the vertical force on a layer cell is proportional to $\mu^{2\mathrm{D}} \mathcal{E} q^2$). For $g$=1 meV/Å$^4$ the peak response of 1 pm/V at a length scale of about 5 nm appears consistent with the measurements of Ref. [25]; an experimental estimate of $g$, together with the Fourier components of the tip potential would be necessary for a more quantitative comparison. By combining the values of $B$ reported in Ref. [24] with the values of $\mu^{2\mathrm{D}}$ calculated in this work (Table I of the main text), one can readily apply Eq. (98) to a broad range of materials of experimental interest.

Note that we have neglected dielectric screening effects in our model. This is an excellent approximation for unsupported 2D layers, since the dielectric function tends to unity [22] in the long-wavelength limit that is relevant to our theory. In the supported case, screening by

the substrate may be important, but this effect can be easily incorporated in the definition of the external electric field, $\mathcal{E}(x, y)$.

## References


[1] David Codony, Irene Arias, and Phanish Suryanarayana. Transversal flexoelectric coefficient for nanostructures at finite deformations from first principles. *Phys. Rev. Materials*, 5(3), March 2021.

[2] M. Stengel. Flexoelectricity from density-functional perturbation theory. *Phys. Rev. B*, 88:174106, 2013.

[3] M. Stengel. Microscopic response to inhomogeneous deformations in curvilinear coordinates. *Nature Communications*, 4:2693, 2013.

[4] Massimiliano Stengel and David Vanderbilt. First-principles theory of flexoelectricity. In Alexander K. Tagantsev and Petr V. Yudin, editors, *Flexoelectricity in Solids From Theory to Applications*, chapter 2, pages 31–110. World Scientific Publishing Co., Singapore, 2016.

[5] X. Gonze and C. Lee. Dynamical matrices, Born effective charges, dielectric permittivity tensors, and interatomic force constants from density-functional perturbation theory. *Phys. Rev. B*, 55:10355, 1997.

[6] Miquel Royo and Massimiliano Stengel. First-principles theory of spatial dispersion: Dynamical quadrupoles and flexoelectricity. *Phys. Rev. X*, 9:021050, Jun 2019.

[7] Andrea Schiaffino, Cyrus E. Dreyer, David Vanderbilt, and Massimiliano Stengel. Metric wave approach to flexoelectricity within density functional perturbation theory. *Phys. Rev. B*, 99:085107, Feb 2019.

[8] X. Gonze, B. Amadon, P.-M. Anglade, J.-M. Beuken, F. Bottin, P. Boulanger, F. Bruneval, D. Caliste, R. Caracas, M. Côté, T. Deutsch, L. Genovese, Ph. Ghosez, M. Giantomassi, S. Goedecker, D.R. Hamann, P. Hermet, F. Jollet, G. Jomard, S. Leroux, M. Mancini, S. Mazevet, M.J.T. Oliveira, G. Onida, Y. Pouillon, T. Rangel, G.-M. Rignanese, D. Sangalli, R. Shaltaf, M. Torrent, M.J. Verstraete, G. Zerah, and J.W. Zwanziger. ABINIT: First-principles approach to material and nanosystem properties. *Computer Phys. Commun.*, 180:2582–2615, 2009.

[9] Miquel Royo, Konstanze R Hahn, and Massimiliano Stengel. Using high multipolar orders to reconstruct the sound velocity in piezoelectrics from lattice dynamics. *Phys. Rev. Lett.*, 125(21):217602, 2020.

[10] D. R. Hamann. Optimized norm-conserving Vanderbilt pseudopotentials. *Phys. Rev. B*, 88:085117, Aug 2013.

[11] M.J. van Setten, M. Giantomassi, E. Bousquet, M.J. Verstraete, D.R. Hamann, X. Gonze, and G.-M. Rignanese. The PseudoDojo: Training and grading a 85 element optimized norm-conserving pseudopotential table. *Comp. Phys. Comm.*, 226:39–54, 2018.

[12] K.S. Novoselov, A. Mishchenko, A. Carvalho, and A.H. Castro Neto. 2d materials and van der waals heterostructures. *Science*, 353(6298):aac9439, July 2016.

[13] Nicholas A. Pike, Benoit Van Troeye, Antoine Dewandre, Guido Petretto, Xavier Gonze, Gian-Marco Rignanese, and Matthieu J. Verstraete. Origin of the counterintuitive dynamic charge in the transition metal dichalcogenides. *Phys. Rev. B*, 95:201106, May 2017.

[14] John P. Perdew, Kieron Burke, and Matthias Ernzerhof. Generalized gradient approximation made simple. *Phys. Rev. Lett.*, 77(18):3865–3868, October 1996.

[15] D.R. Hamann, Karin M. Rabe, and David Vanderbilt. Generalized-gradient-functional treatment of strain in density-functional perturbation theory. *Phys. Rev. B*, 72(3), July 2005.

[16] Xiaoying Zhuang, Bo He, Brahmanandam Javvaji, and Harold S. Park. Intrinsic bending flexoelectric constants in two-dimensional materials. *Phys. Rev. B*, 99:054105, Feb 2019.

[17] T. Pandey, L. Covaci, and F.M. Peeters. Tuning flexoelectricty and electronic properties of zig-zag graphene nanoribbons by functionalization. *Carbon*, 171:551–559, January 2021.

[18] T. Pandey, L. Covaci, M. V. Milošević, and F. M. Peeters. Flexoelectricity and transport properties of phosphorene nanoribbons under mechanical bending. *Phys. Rev. B*, 103:235406, Jun 2021.

[19] Brahmanandam Javvaji, Bo He, Xiaoying Zhuang, and Harold S. Park. High flexoelectric constants in janus transition-metal dichalcogenides. *Phys. Rev. Materials*, 3:125402, Dec 2019.

[20] Wenhao Shi, Yufeng Guo, Zhuhua Zhang, and Wanlin Guo. Flexoelectricity in monolayer transition metal dichalcogenides. *The Journal of Physical Chemistry Letters*, 9(23):6841–6846, 12 2018.

[21] Anubhav Jain, Shyue Ping Ong, Geoffroy Hautier, Wei Chen, William Davidson Richards, Stephen Dacek, Shreyas Cholia, Dan Gunter, David Skinner, Gerbrand Ceder, and Kristin A. Persson. The materials project: A materials genome approach to accelerating materials innovation. *APL Materials*, 1(1):011002, July 2013.

[22] Miquel Royo and Massimiliano Stengel. Exact long-range dielectric screening and interatomic force constants in quasi-2d crystals. *Physical Review X (accepted), arXiv preprint arXiv:2012.07961*, 2020.

[23] Bruno Amorim and Francisco Guinea. Flexural mode of graphene on a substrate. *Phys. Rev. B*, 88:115418, Sep 2013.

[24] Shashikant Kumar and Phanish Suryanarayana. Bending moduli for forty-four select atomic monolayers from first principles. *Nanotechnology*, 31(43):43LT01, aug 2020.

[25] Christopher J. Brennan, Rudresh Ghosh, Kalhan Koul, Sanjay K. Banerjee, Nanshu Lu, and Edward T. Yu. Out-of-plane electromechanical response of monolayer molybdenum disulfide measured by piezoresponse force microscopy. *Nano Letters*, 17(9):5464–5471, 09 2017.
